# Supplementary material for: Representing Volumetric Videos as Dynamic MLP Maps
Source: arXiv:2304.06717 source file (2023-04-13)
Supplement: Supplementary file 1 [file comparison_baselines.tex]

\vspace{-0.8em}
\begin{table}[!htbp]
\begin{center}
\scalebox{0.66}{
\begin{tabular}{x{42}|x{68}x{64}x{63}x{55}}
Methods & Baseline1 & C-NeRF & Ours-Single & Ours \\[.1em]
\shline
\multirow{2}{*}{Description} & feature tri-planes + single NeRF & feature volumes + single NeRF & hash tables + single NeRF & hash tables + MLP maps \\ \hline
LPIPS & 0.065 & 0.057 & 0.056 & \textbf{0.049}
\end{tabular}
} % scalebox
\vspace{-1.8em}
\end{center}
\caption{Comparison on the ``Twirl'' subject of ZJU-MoCap.}
\vspace{-2mm}
\label{tab:comparison_baselines}
\end{table}
