# Supplementary material for: Representing Volumetric Videos as Dynamic MLP Maps
Source: arXiv:2304.06717 source file (2023-04-13)
Supplement: Supplementary file 2 [file rendering_speed.tex]

\vspace{-0.8em}
\begin{table}[!htbp]
\begin{center}
\scalebox{0.70}{
\begin{tabular}{c|ccc}
& Single MLP w/o ESS & MLP maps w/o ESS & Complete \\[.1em]
\shline
Rendering time (ms) & 1345 & 144 & 24
\end{tabular}
} % scalebox
\vspace{-1.8em}
\end{center}
\caption{Results are obtained from Table 1 (6, 9, 10).}
\vspace{-2mm}
\label{tab:rendering_speed}
\end{table}
